# Supplementary material for: Charge-transfer steps in Density Functional Theory from the perspective of the Exact Electron Factorization
Source: arXiv:2101.07858 ancillary file (2021-03-22)
Supplement: Supplementary file 1 [file paper_letter_v4_si.pdf]

# Supplemental material for "Charge-transfer steps in Density Functional Theory from the perspective of the Exact Electron Factorization"

Jakub Kocák,† Eli Kraisler,‡ and Axel Schild*,†

†*Laboratorium für Physikalische Chemie, ETH Zürich, Vladimir-Prelog-Weg 2, 8093 Zürich, Switzerland*

‡*Fritz Haber Center for Molecular Dynamics, Institute of Chemistry, The Hebrew University of Jerusalem, 91904 Jerusalem, Israel*

E-mail: axel.schild@phys.chem.ethz.ch

The one-dimensional model considered in our letter represents a diatomic with external potential provided by a nucleus of charge +2 and a nucleus with charge +1. In the letter, the totally antisymmetric spatial state for two electrons is considered, as its conditional wavefunction $\phi(x_2; x_1)$ can be plotted easily.

We also investigated the totally antisymmetric spatial state for three electrons. Fig. 1 shows the relevant quantities for an internuclear distance $R = 10\,a_0$. The three lowest Kohn-Sham (KS) orbitals $\varphi_j^{\mathrm{KS}}$ of the KS potential $v^{\mathrm{KS}}$ are each occupied by one electron. Orbitals $\varphi_0^{\mathrm{KS}}$ and $\varphi_2^{\mathrm{KS}}$ are localized on the (left) nucleus with charge +2, while $\varphi_1^{\mathrm{KS}}$ is localized on the (right) nucleus with charge +1.

The exact electron factorization (EEF) potentials are similar to their KS counterparts, i.e.,

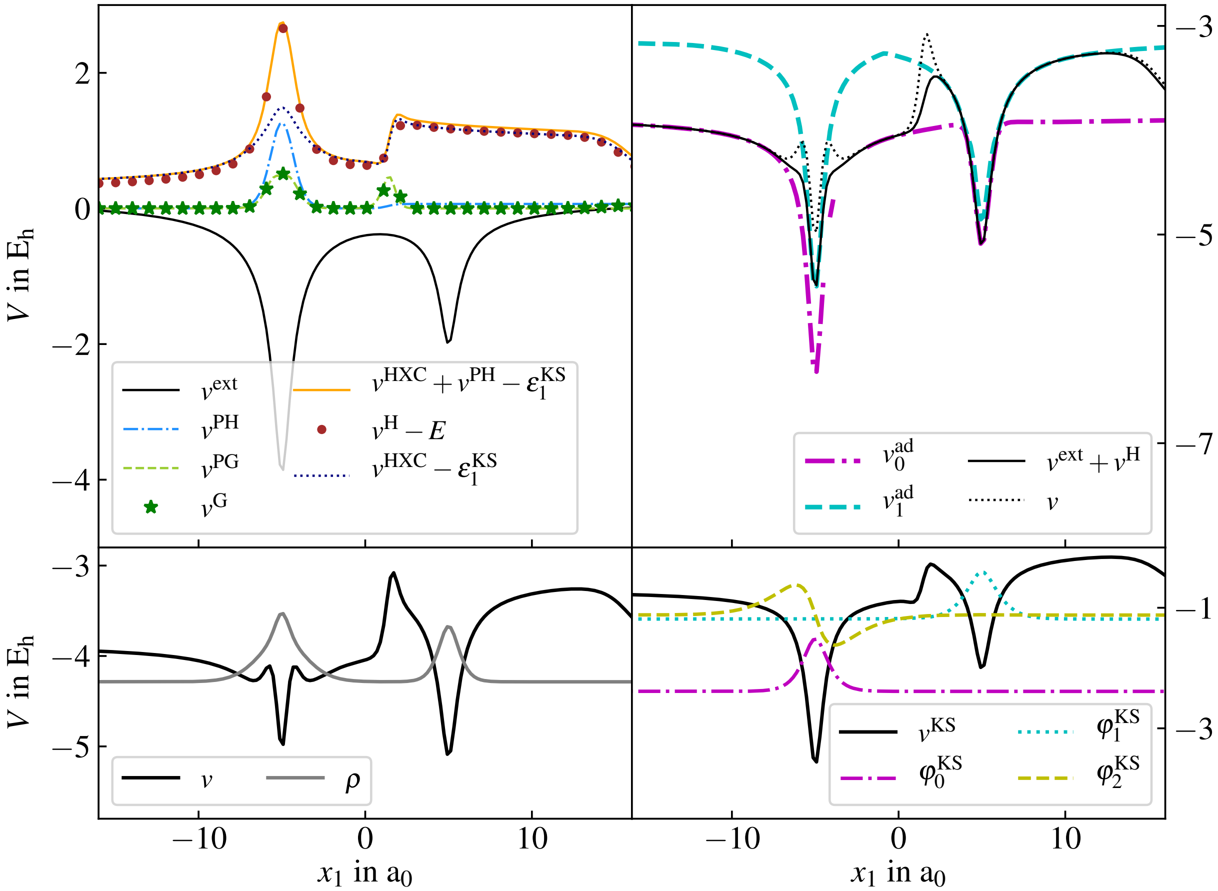


Figure 1: one-electron quantities for the model of the heteronuclear diatomic with three electrons. Top left: External potential $v^{\mathrm{ext}}$ and contributions to the EEF potential $v$ based on the interacting system ($v^{\mathrm{H}}$ and $v^{\mathrm{G}}$) and on the KS system ($v^{\mathrm{HXC}}$, $v^{\mathrm{PH}}$, and $v^{\mathrm{PG}}$). Top right: EEF potential $v$ and $v^{\mathrm{ext}} + v^{\mathrm{H}} = v - v^{\mathrm{G}}$ as well as the lowest two adiabatic potentials $v_j^{\mathrm{ad}}$ for states with the correct symmetry. Bottom left: EEF potential $v$ and one-electron density $\rho$ (shifted to the energy $E$ of the state). Bottom right: KS potential $v^{\mathrm{KS}}$ and occupied KS orbitals $\varphi_j^{\mathrm{KS}}$ (shifted to their eigenvalues $\varepsilon_j^{\mathrm{KS}}$).

$v^{\mathrm{H}} \approx v^{\mathrm{HXC}} + v^{\mathrm{PH}}$ and $v^{\mathrm{G}} \approx v^{\mathrm{PG}}$, up to a constant. The average energy of the conditioned (two-electron) system $v^{\mathrm{H}}$ is bell-shaped around the nucleus of charge +2 and has a step in the internuclear region, leading to a plateau on the side of the nucleus with charge +1 that ends for larger values of $x_1$. The geometric potential $v^{\mathrm{G}}$ is non-zero and bell-shaped around the nucleus of charge +2 and the step up to the plateau in $v^{\mathrm{H}}$. It is also a wide and shallow bell around the step down from the plateau in $v^{\mathrm{H}}$, which is, however, barely visible in the figure. The interpretation of these features is the same as discussed in our letter, with the additional complication that, at the nucleus with charge +2, there is now a two-electron atom. The electron-electron interaction there gives rise to the bell-shaped features of the potentials at that nucleus.

Like for the two-electron model, the potential $v^{\mathrm{ext}} + v^{\mathrm{H}} = v - v^{\mathrm{G}}$ is piecewise composed of the lowest two potentials $v_j^{\mathrm{ad}}$ of the adiabatic states with correct symmetry, i.e., $\phi_j^{\mathrm{ad}}(2,3;1) = -\phi_j^{\mathrm{ad}}(3,2;1)$.
